# Supplementary material for: The Importance of Non-Markovianity in Maximum State Entropy Exploration
Source: arXiv:2202.03060 source file (2022-07-08)
Supplement: Supplementary file 1 [file appendix_additional_results.tex]

Throughout the paper, we mostly considered the class of non-Markovian policies against the class of Markovian policies. However, one could wonder how non-stationary policies fare in dealing with the finite-sample MSE objective~\eqref{eq:finite_samples_entropy}. Here we would like to report some informal results on this point.
On the one hand, non-stationary policies have a clear edge over stationary Markovian policies, as they can adapt the strategy in a state $s \in \Sspace$ encountered at different steps. However, they still cannot fully resolve the partial observability over the current history. This uncertainty over the history arguably induces some positive regret-to-go \wrt non-Markovian policies.
Especially, one would expect that an optimal non-stationary policy $\pi_{\NS} \in \argmax_{\pi \in \Pins} \mathcal{E} (\pi)$ could be randomized in order to cope with this uncertainty, and thus that the result of Lemma~\ref{thr:law_total_variance} could be extended as
\begin{equation*}
	\Var \big[ \mathcal{B} ( \pi_{\NS} (a^*|s, t) ) \big] = \Var_{hs \sim p^{\pi_{\NM}}_t} \big[ \EV \big[ \mathcal{B} ( \pi_{\NM} (a^* | hs) ) \big] \big],
\end{equation*}
where $hs$ is any history of $t$ steps $hs \in \Hspace_t$ such that the final state is $s$, instead of any history of any length $hs \in \Hspace_{[T]}$ terminating in $s$ as in Lemma~\ref{thr:law_total_variance}. The last result could be plugged in upper and lower bounds to the regret-to-go similar to Lemma~\ref{thr:regret_bounds}, and corresponding Theorem~\ref{thr:regret_theorem} and Corollary~\ref{thr:sufficient_condition} should be easily extended to non-stationary policies. Finally, although an optimal non-stationary policy $\pi_{\NS}$ would not be zero-regret in general, it could suffer a lower regret than an optimal Markovian policy. Formally establishing this regret gap might be an interesting direction for future works.

To assess the importance of non-Markovianity in MSE exploration, we adopted the most common state distribution formulation. As we mentioned in Appendix~\ref{apx:related_work}, other works in the MSE literature considered the entropy of the state-action distribution in the objective function. Analogously, we can recast the finite-sample objective as $\EV_{h \sim p_{T}^{\pi}} [ H (d_h (\cdot, \cdot))]$ and replicate most of the results that we reported in the paper. In this alternative formulation, the class of non-Markovian policies would still preserve an edge over the classes of non-stationary and Markovian policies. Accounting for the entropy of the state-action distribution might be crucial in the settings where the exploration over the action space cannot be overlooked (\eg a single-trial setting).
